# Supplementary material for: HCV: Hierarchy-Consistency Verification for Incremental Implicitly-Refined Classification
Source: arXiv:2110.11148 source file (2021-10-22)
Supplement: Supplementary file 2 [file supp.pdf]

# Supplementary materials for HCV: Hierarchy-Consistency Verification for Incremental Implicitly-Refined Classification

Kai Wang<sup>1</sup>

kwang@cvc.uab.es

Xialei Liu<sup>2</sup>

xialei@nankai.edu.cn

Luis Herranz<sup>1</sup>

lherranz@cvc.uab.es

Joost van de Weijer<sup>1</sup>

joost@cvc.uab.es

<sup>1</sup> Computer Vision Center

Universitat Autònoma de Barcelona

Barcelona, Spain

<sup>2</sup> College of Computer Science

Nankai University

Tianjin, China

---

## 1 Confusion matrices

Fig. 7 and Fig. 8 show the confusion matrices after learning task 11 and the last task under IIRC-2-CIFAR setup. We can observe similar trends as in Fig. 5 in the main paper when applying the HCV modules to training and inference stages of iCaRL-CNN.

## 2 Infer-HCV

We verify the hierarchy consistency also at inference time (see Section 3.2). Here we provide some examples for better understanding of Infer-HCV. In Fig. 9 there are four examples of how the *Infer-HCV* module works. We address the examples one column at a time:

- I. This example is correctly matched by the first row of  $H_t$ , so it remains unchanged.
- II. This example does not match any row in  $H_t$ . We match it with the first row by removing the second label.
- III. This example also does not match. We match it by adding the first class label to make it in accordance with the last row of  $H_t$ .
- IV. This example also does not match. It can be modified by removing the 4th or 5th labels, so we randomly choose one from them to make it compatible with  $H_t$ .

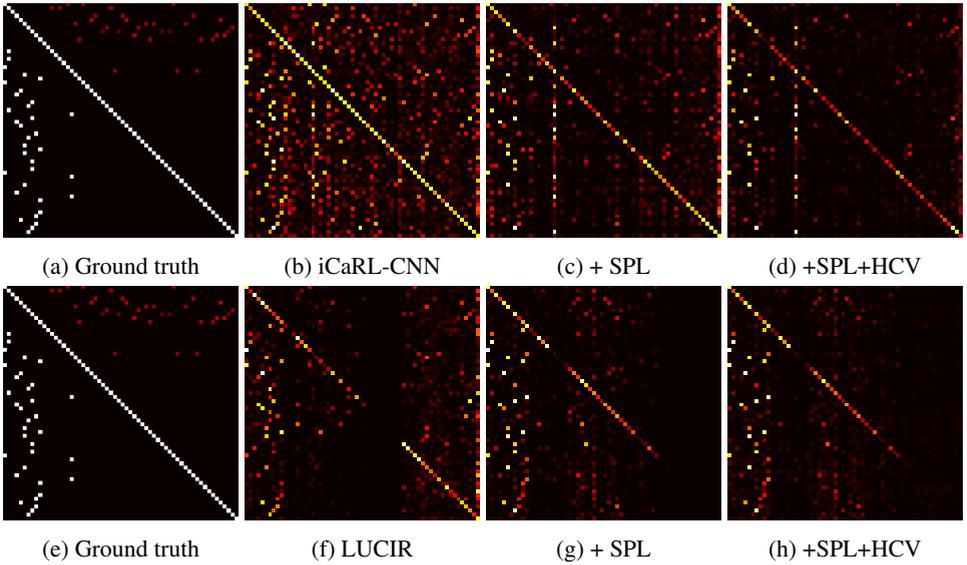

Figure 7: Confusion matrices of groundtruth, original continual learning methods, applying SPL and applying Infer-HCV after task 11 under IIRC-2-CIFAR setup. The first row is obtained with iCaRL-CNN as the base method and the second row is based on LUCIR.

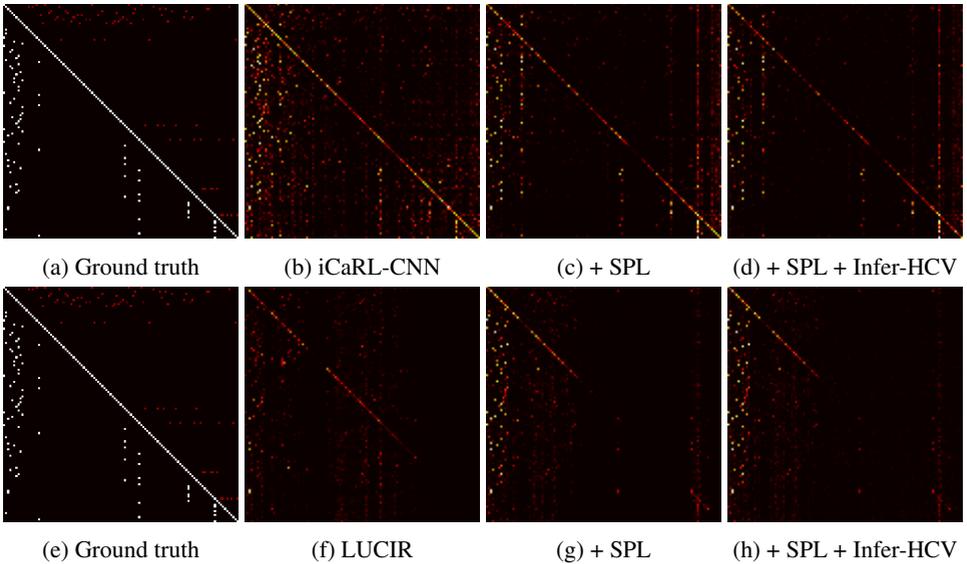

Figure 8: Confusion matrices of groundtruth, original continual learning methods, applying SPL and applying Infer-HCV after the last task under IIRC-2-CIFAR setup. The first row is obtained with iCaRL-CNN as the base continual learning method and the second row is based on LUCIR.

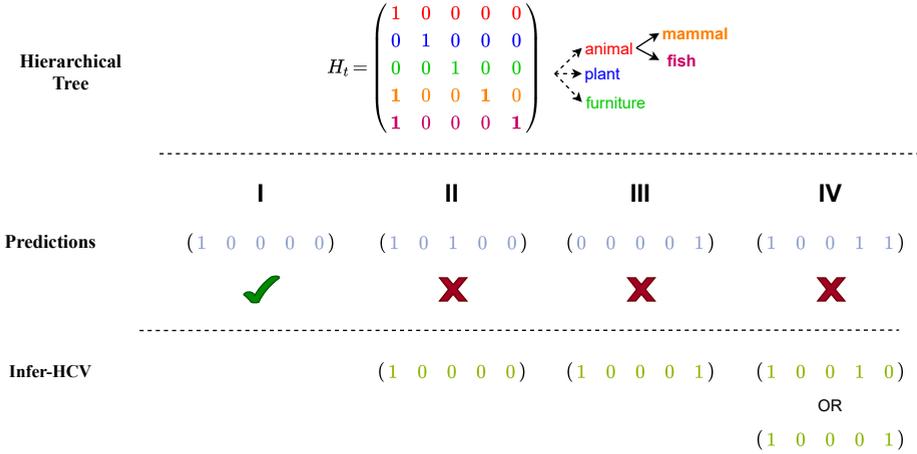

Figure 9: Examples Illustration of Infer-HCV procedure.

### 3 Groundtruth hierarchies and task splits

Here we show the groundtruth hierarchies of IIRC-2-CIFAR/IIRC-3-CIFAR in Table 1 and IIRC-ImageNet-Subset in Table 2. For the task splits used in our experiments, we select one from the IIRC paper for IIRC-2-CIFAR (Table 3) and propose our splits for IIRC-3-CIFAR (Tab. 4)/IIRC-ImageNet-Subset (Tab. 5) to test the models in more complex hierarchies.

### 4 Experimental results for IIRC-ImageNet-full

In Fig. 10 we show results for the first 20 tasks (out of 35 in total)<sup>1</sup> for LUCIR and iCaRL-CNN. Our HCV improves by 4.2% for LUCIR and 1.9% for iCaRL-CNN after 20 tasks.

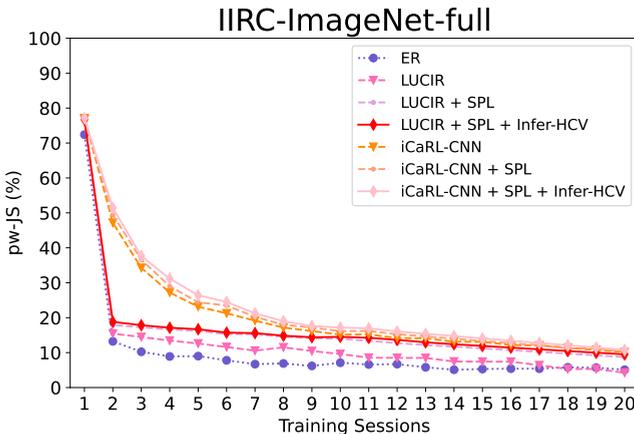

Figure 10: Experiments for IIRC-ImageNet-full.

<sup>1</sup>Because of the demanding computational resources required for this experiment we were only able to compute results until task 20.

| rootclass | superclass                     | subclasses                                                                                                                                                                         |
|-----------|--------------------------------|------------------------------------------------------------------------------------------------------------------------------------------------------------------------------------|
| animals   | aquatic mammals                | beaver,dolphin,otter,seal,whale                                                                                                                                                    |
|           | fish                           | aquarium fish,flatfish,ray,shark,trout                                                                                                                                             |
|           | insects                        | bee,beetle,butterfly,caterpillar,cockroach                                                                                                                                         |
|           | large carnivores               | leopard,lion,tiger,wolf                                                                                                                                                            |
|           | large omnivores and herbivores | bear,camel,cattle,chimpanzee,elephant,kangaroo                                                                                                                                     |
|           | medium sized mammals           | fox,porcupine,possum,raccoon,skunk                                                                                                                                                 |
|           | reptiles                       | crocodile,dinosaur,lizard,snake,turtle                                                                                                                                             |
| plants    | small mammals                  | hamster,mouse,rabbit,shrew,squirrel                                                                                                                                                |
|           | flowers                        | orchid,poppy,rose,sunflower,tulip                                                                                                                                                  |
|           | fruit and vegetables           | apple,orange,pear,sweet pepper                                                                                                                                                     |
| -         | trees                          | maple tree,oak tree,palm tree,pine tree,willow tree                                                                                                                                |
|           | vehicles                       | bicycle,bus,motorcycle,pickup truck,<br>train,streetcar,tank,tractor                                                                                                               |
|           | household furniture            | bed,chair,couch,table,wardrobe                                                                                                                                                     |
|           | food containers                | bottle,bowl,can,cup,plate                                                                                                                                                          |
| -         | people                         | baby,boy,girl,man,woman                                                                                                                                                            |
| -         | -                              | mushroom,clock,keyboard,lamp,telephone,<br>television,bridge,castle,house,road,<br>skyscraper,cloud,forest,mountain,plain,<br>sea,crab,lobster,snail,spider,worm,lawn mower,rocket |

Table 1: IIRC-2-CIFAR and IIRC-3-CIFAR Hierarchies. IIRC-2-CIFAR is without the root-classes.

| superclass | subclasses                                                                                                                                                                                                        |
|------------|-------------------------------------------------------------------------------------------------------------------------------------------------------------------------------------------------------------------|
| primate    | Madagascar cat, indri, gibbon, siamang, orangutan, gorilla, chimpanzee, marmoset, capuchin, howler monkey,titi, spider monkey, squirrel monkey, guenon, patas, baboon, macaque, langur, colobus, proboscis monkey |
| car        | ambulance, beach wagon, cab, convertible, jeep, limousine, Model T, racer, sports car, minivan, grille, golfcart                                                                                                  |
| ball       | baseball, basketball, croquet ball, golf ball, ping-pong ball, punching bag, rugby ball, soccer ball, tennis ball, volleyball                                                                                     |
| crustacean | isopod, crayfish, hermit crab, spiny lobster, American lobster, Dungeness crab, rock crab, fiddler crab, king crab                                                                                                |
| weapon     | bow, projectile, cannon, missile, rifle, revolver, assault rifle, holster bison,                                                                                                                                  |
| spider     | black and gold garden spider, barn spider, garden spider, black widow, tarantula, wolf spider, spider web                                                                                                         |
| box        | carton, chest, crate, mailbox, pencil box, safe                                                                                                                                                                   |
| bag        | backpack, mailbag, plastic bag, purse, sleeping bag                                                                                                                                                               |
| beverage   | espresso, red wine, cup, eggnog                                                                                                                                                                                   |
| keyboard   | computer keyboard, space bar, typewriter keyboard                                                                                                                                                                 |
| -          | African crocodile, American alligator, triceratops, trilobite, harvestman, scorpion, tick, centipede, tusker, echidna, platypus, jellyfish, sea anemone, brain coral, flatworm, nematode                          |

Table 2: IIRC-ImageNet-Subset Hierarchy

| Task ID | Classes                                                                                                                                                                    |
|---------|----------------------------------------------------------------------------------------------------------------------------------------------------------------------------|
| 1       | flowers (S), small mammals (S), trees (S), aquatic mammals (S), fruit and vegetables (S), people (S), food containers (S), vehicles (S), large carnivores (S), insects (S) |
| 2       | television, spider, shrew, mountain, hamster                                                                                                                               |
| 3       | road, poppy, household furniture (S), woman, bee                                                                                                                           |
| 4       | tulip, clock, orange, beaver, rocket                                                                                                                                       |
| 5       | bicycle, can, squirrel, wardrobe, bus                                                                                                                                      |
| 6       | whale, sweet pepper, telephone, leopard, bowl                                                                                                                              |
| 7       | skyscraper, baby, cockroach, boy, lobster                                                                                                                                  |
| 8       | motorcycle, forest, tank, orchid, chair                                                                                                                                    |
| 9       | crab, girl, keyboard, otter, bed                                                                                                                                           |
| 10      | butterfly, lawn mower, snail, caterpillar, wolf                                                                                                                            |
| 11      | pear, tiger, pickup truck, cup, reptiles (S)                                                                                                                               |
| 12      | train, sunflower, beetle, apple, palm tree                                                                                                                                 |
| 13      | plain, large omnivores and herbivores (S), rose, tractor, crocodile                                                                                                        |
| 14      | mushroom, couch, lamp, mouse, bridge                                                                                                                                       |
| 15      | turtle, willow tree, man, lizard, maple tree                                                                                                                               |
| 16      | lion, elephant, seal, sea, dinosaur                                                                                                                                        |
| 17      | worm, bear, castle, plate, dolphin                                                                                                                                         |
| 18      | medium sized mammals (S), streetcar, bottle, kangaroo, snake                                                                                                               |
| 19      | house, chimpanzee, raccoon, porcupine, oak tree                                                                                                                            |
| 20      | pine tree, possum, skunk, fish (S), fox                                                                                                                                    |
| 21      | cattle, ray, aquarium fish, cloud, flatfish                                                                                                                                |
| 22      | rabbit, trout, camel, table, shark                                                                                                                                         |

Table 3: IIRC-2-CIFAR task split configuration. (S) denotes the super classes.

| Task ID | Classes                                                                        |
|---------|--------------------------------------------------------------------------------|
| 1       | <b>animals (R)</b> , food containers (S), house, road, telephone, lamp, rocket |
| 2       | fish (S), crab, snail, mushroom, bottle                                        |
| 3       | reptiles (S), sea, trout, can, clock                                           |
| 4       | vehicles (S), flatfish, snake, aquarium fish, mountain                         |
| 5       | large omnivores and herbivores (S), plate, cup, television, ray                |
| 6       | small mammals (S), camel, bicycle, keyboard, lawn mower                        |
| 7       | household furniture (S), shark, turtle, spider, forest                         |
| 8       | aquatic mammals (S), couch, kangaroo, streetcar, lobster                       |
| 9       | insects (S), tank, plain, motorcycle, whale                                    |
| 10      | large carnivores (S), bear, crocodile, dinosaur, otter                         |
| 11      | <b>plants (R)</b> , medium sized mammals (S), tractor, table, bowl             |
| 12      | fruit and vegetables (S), chimpanzee, cloud, raccoon, butterfly                |
| 13      | flowers (S), bus, shrew, wardrobe, apple                                       |
| 14      | people (S), mouse, skunk, caterpillar, castle                                  |
| 15      | trees (S), fox, cockroach, worm, squirrel                                      |
| 16      | palm tree, oak tree, lizard, maple tree, orchid                                |
| 17      | rose, bed, train, elephant, sweet pepper                                       |
| 18      | skyscraper, beetle, boy, pine tree, lion                                       |
| 19      | hamster, pear, bee, man, tiger                                                 |
| 20      | seal, poppy, porcupine, dolphin, tulip                                         |
| 21      | orange, wolf, cattle, willow tree, woman                                       |
| 22      | bridge, pickup truck, baby, sunflower, girl                                    |
| 23      | leopard, rabbit, beaver, possum, chair                                         |

Table 4: IIRC-3-CIFAR task split configuration. (R) denotes the root classes and (S) denotes the super classes.

| Task ID | Classes                                                                                                                                 |
|---------|-----------------------------------------------------------------------------------------------------------------------------------------|
| 1       | car (S), box (S), brain coral, echidna, American alligator, African crocodile, tusker, jellyfish, sea anemone, tick                     |
| 2       | bag (S), crustacean (S), trilobite, ambulance, triceratops, sports car, mailbox, grille, nematode, limousine                            |
| 3       | weapon (S), pencil box, jeep, Model T, purse, mailbag, hermit crab, centipede, beach wagon, fiddler crab                                |
| 4       | beverage (S), safe, minivan, scorpion, assault rifle, harvestman, missile, sleeping bag, holster, projectile                            |
| 5       | keyboard (S), revolver, Dungeness crab, American lobster, king crab, cab, convertible, racer, isopod, chest                             |
| 6       | ball (S), backpack, cannon, crayfish, rock crab, espresso, platypus, flatworm, rifle, space bar                                         |
| 7       | spider (S), spiny lobster, volleyball, punching bag, carton, golfcart, plastic bag, golf ball, eggnog, baseball                         |
| 8       | primate (S), black widow, basketball, typewriter keyboard, bow, tarantula, garden spider, rugby ball, cup, black and gold garden spider |
| 9       | wolf spider, marmoset, squirrel, monkey, guenon, orangutan, macaque, baboon, Madagascar cat, capuchin, soccer ball                      |
| 10      | howler monkey, siamang, gibbon, gorilla, spider web, red wine, crate, colobus, tennis ball, barn spider                                 |
| 11      | croquet ball, indri, chimpanzee, titi, spider monkey, langur, ping-pong ball, computer keyboard, patas, proboscis monkey                |

Table 5: IIRC-ImageNet-Subset task split configuration. (S) denotes the super classes.
